# Supplementary material for: Differentially Encoded Observation Spaces for Perceptive Reinforcement Learning
Source: arXiv:2310.01767 source file (2023-10-03)
Supplement: Supplementary file 1 [file 7_appendix.tex]

\todo{Update}

% \textbf{Learning Hyperparameters:} 
% All experiments were carried out using the default $\texttt{stable-baselines3}$ learning parameters for PPO and SAC unless otherwise noted. The full hyperparameter list is given in Table~\ref{table:hyperparameters}. Both PPO and SAC used two-layered feed-forward networks with 64 nodes per layer.

% \begin{table}[h!]
% \centering
% \bgroup
% \def\arraystretch{1.2} % Add more vertical spacing.
% \begin{tabular}{ |l|l|c| }
%   \hline
%   & Parameter & Value \\
%   \hline
%    \multirow{8}{2em}{PPO} & MDP steps per update& 2048\\
% %  \hline
%    & batch size & 64\\
%    & learning rate & 0.0003\\
% %  \hline
%    & gamma & 0.99\\
%    & $\lambda$ for GAE & 0.95\\
% %  \hline
%    & value function cost & 0.5\\
% %  \hline
%    & entropy cost & 0.0\\
% %  \hline
%    & max gradient norm & 0.5\\
% %  \hline
% %  \hline
%    & cliprange & 0.2\\
%  \hline
%    \multirow{7}{2em}{SAC} & learning rate & 0.0003\\
%    & buffer size & 1000000\\
%    & entropy coefficient & auto\\
%    & MDP steps between updates & 1\\
%    & batch size & 256\\
%    & tau & 0.005\\
%    & gamma & 0.99\\
%    & gradient steps per update & 1\\
%  \hline
% \end{tabular}
% \egroup
% \caption{Learning hyperparameters}
% \label{table:hyperparameters}
% \vspace{-10pt}
% \end{table}
